# Supplementary material for: Multidimensional Eigenwave Multiplexing Modulation for Non-Stationary Channels
Source: arXiv:2211.09203 source file (2023-08-30)
Supplement: Supplementary file 1 [file appendix.tex]

\appendices
\label{appendix:MEM}

\section{Statistics of non-stationary channels}
% \ingreen{Maqsood: I will show the $h(t,\tau)$ and $L_H(t,f)$ figures and they can both show NS. It's better to explain (6) and (7) by $h(t,\tau)$ instead of $S_H$.}
% \noindent
% % \note{Is it needed:}

For stationary channels, the TF transfer function is a stationary process and and the spreading function is a white process (uncorrelated scattering) which are related as,
\begin{equation}
    \mathbb{E}\{L_H(t, f) L_H^*(t',f')\} {=} R_H(t{-}t',f{-}f')
\end{equation}

\begin{equation}
    \mathbb{E}\{S_H(\tau, \nu) S_H^*(\tau',\nu')\} {=} C_H(\tau,\nu) \delta (\tau{-} \tau') \delta(\nu{-} \nu')
\end{equation}

where $\delta(\cdot)$ is the Dirac delta function.
$C_H(\tau,\nu)$ and $R_H(t-t',f-f')$ are the \textit{scattering function} and \textit{TF correlation function}, respectively, which are related via 2-D Fourier transform, 

% For stationary channels, the TF transfer function is a stationary process andwith $\mathbb{E}\{L_H(t, f) L_H^*(t',f')\} {=} R_H(t{-}t',f{-}f')$, and the spreading function is a white process (uncorrelated scattering), i.e., $\mathbb{E}\{S_H(\tau, \nu) S_H^*(\tau',\nu')\} {=} C_H(\tau,\nu) \delta (\tau{-} \tau') \delta(\nu{-} \nu')$, where $\delta(\cdot)$ is the Dirac delta function.
% $C_H(\tau,\nu)$ and $R_H(t-t',f-f')$ are the \textit{scattering function} and \textit{TF correlation function}, respectively, which are related via 2-D Fourier transform, 
% as,
% \textbf{WSSUS channel:} 1) TF transfer function is a stationary process with $\mathbb{E}\{L_H(t, f) L_H^*(t',f')\} {=} R_H(t-t',f-f')$. 2) Spreading function is a white process (uncorrelated scattering), i.e., $\mathbb{E}\{S_H(\tau, \nu) S_H^*(\tau',\nu')\} {=} C_H(\tau,\nu) \delta (\tau{-} \tau') \delta(\nu{-} \nu')$ .
% $C_H(\tau,\nu)$ and $R_H(t-t',f-f')$ are \textit{scattering function} and \textit{TF correlation function}, respectively, which are related via 2-D Fourier transform
% \useshortskip
\begin{equation}
    C_H(\tau,\nu) = \iint R_H(\Delta t, \Delta f) e^{-j2\pi(\nu \Delta t -  \tau \Delta f)} ~d\Delta t ~d\Delta f
\end{equation}
% \noindent
% \textbf{Non-WSSUS channel:}
In contrast, for non-stationary channels, the TF transfer function is a non-stationary process and the spreading function is a non-white process. %Since $C_H(\tau,\nu)$ is not defined for non-WSSUS channel, 
Therefore, a \textit{local scattering function} (LSF) $\mathcal{C}_H(t,f;\tau,\nu)$ \cite{Matz2005NS} is defined to extend $C_H(\tau,\nu)$ to non-stationary channels in \eqref{eq:LSF}. 
Similarly, the \textit{channel correlation function} (CCF) $\mathcal{R}(\Delta t, \Delta f;\Delta \tau, \Delta \nu)$ generalizes $R_H(\Delta t, \Delta f)$ to the non-stationary case in \eqref{eq:CCF}.
\begin{align}
\begin{split}
    &\mathcal{C}_H(t,f ; \tau,\nu)  \label{eq:LSF}\\
    & {=} {\iint} R_L(t, f; \Delta t, \Delta f) e^{-j2\pi(\nu \Delta t -  \tau \Delta f)} ~d\Delta t ~d\Delta f  \\
    & {=} \iint R_S(\tau, \nu; \Delta \tau, \Delta \nu) e^{-j2\pi(t \Delta \nu -  f \Delta \tau)} ~d\Delta \tau ~d\Delta \nu \\
\end{split}\\
\begin{split}
    &\mathcal{R}(\Delta t, \Delta f;\Delta \tau, \Delta \nu) \label{eq:CCF}\\
    & {=} \iint R_L(t, f; \Delta t, \Delta f) e^{-j2\pi(\Delta \nu  t -  \Delta \tau  f)} ~d t ~d f \\
    & {=} \iint R_S(\tau, \nu; \Delta \tau, \Delta \nu) e^{-j2\pi(\Delta t \nu -  \Delta f  \tau)} ~d \tau ~d \nu
\end{split}
\end{align}
where, $R_L(t, f; \Delta t, \Delta f)=\mathbb{E}\{L_H(t, f {+} \Delta f) L_H^*(t {-} \Delta t, f)\}$ and $R_S(\tau, \nu; \Delta \tau, \Delta \nu)=\mathbb{E}\{S_H(\tau, \nu {+} \Delta \nu) S_H^*(\tau{-} \Delta \tau, \nu)\}$. 
For stationary channels, CCF reduces to TF correlation function $\mathcal{R}(\Delta t, \Delta f;\Delta \tau, \Delta \nu){=}R_H(\Delta t, \Delta f) \delta(\Delta t) \delta(\Delta f)$.

\section{Proof of Lemma 1: Associative property of eigenwave set projectio}
\label{app:Proof_MEM}

% \subsection{Proof of Lemma 1: Associative property of eigenwave set projectio}
\label{App:Ass}
% \begin{lemma}
% (Associative property of eigenwave set projection) Define $\Phi_{a} = \Sigma_n^N a_n \phi_n (\gamma_1{,}{...}{,}\gamma_Q)$, we have
% \begin{align}
%     \langle \Phi_a ,\Phi_b^*\rangle = \langle\Phi_{ab}, \Phi^*\rangle = \langle \Phi , \Phi_{ab}^*\rangle
% \end{align}
% where $\langle \cdot, \cdot \rangle$ is the eigenwave set projection operator. $\phi_n(\gamma_1{,}{...}{,}\gamma_Q)$ is $Q$ dimensional eigenfunction.
% \end{lemma}
\begin{proof}

\begin{align}
    & \langle \Phi_a ,\Phi_b^*\rangle = \int{...}\int  \Sigma_n^N a_n \phi_n (\gamma_1{,}{...}{,}\gamma_Q) \Sigma_n^N b_n \phi_n^* (\gamma_1{,}{...}{,}\gamma_Q)\nonumber \\ & ~d\gamma_1 {,}{...}{,} ~d\gamma_Q \nonumber \\ \nonumber
    & = \int{...}\int \Sigma_n^N a_n \phi_n (\gamma_1{,}{...}{,}\gamma_Q) b_n \phi_n^* (\gamma_1{,}{...}{,}\gamma_Q) ~d\gamma_1 {,}{...}{,} ~d\gamma_Q \nonumber \\
    & + \underbrace{\int{...}\int \Sigma_{n' \neq n }^N a_n b_{n'} \phi_n(\gamma_1{,}{...}{,}\gamma_Q) \phi_{n'}^*(\gamma_1{,}{...}{,}\gamma_Q) ~d\gamma_1 {,}{...}{,} ~d\gamma_Q}_{=0} \nonumber  \\ 
    & = \int{...}\int \Sigma_n^N a_n b_n \phi_n (\gamma_1{,}{...}{,}\gamma_Q) \phi_n^*(\gamma_1{,}{...}{,}\gamma_Q) ~d\gamma_1 {,}{...}{,} ~d\gamma_Q  \nonumber  \\ 
    & = \int{...}\int \Sigma_n^N a_n b_n \phi_n (\gamma_1{,}{...}{,}\gamma_Q) \Sigma_n ^N \phi_n^*(\gamma_1{,}{...}{,}\gamma_Q) ~d\gamma_1 {,}{...}{,} ~d\gamma_Q \nonumber \\ 
    & = \langle \Phi_{ab} ,\Phi^*\rangle
\end{align}

From a similar deduction, we also have $\langle \Phi_a ,\Phi_b^*\rangle = \langle \Phi ,\Phi_{ab}^*\rangle$
\end{proof}

\section{Deduction of (22)}
\label{app:deduc_22}

\begin{align}
   & \iiiint |h_w(t,f;\tau,\nu)|^2~dt~df~d\tau~d\nu \nonumber \\ \nonumber
   {=} & \iiiint \left |\sum_n^N \sigma_n \phi_n(t,f) \psi_n(\tau,\nu)  \right|^2~dt~df~d\tau~d\nu \\ \nonumber
   {=} & \iiiint \sum_n^N \sigma_n^2 \underbrace{|\phi_n(t,f)|^2}_{{=}1} \underbrace{|\psi_n(\tau,\nu)|^2}_{{=}1}  \\ \nonumber
   {+} & \underbrace{ \sum_{n^\prime \neq n}^N \sigma_n \sigma_{n^\prime} \phi_n(t,f) \phi_{n^\prime} (t,f)^* \psi_n(\tau,\nu) \psi_{n^\prime}(\tau,\nu)^*}_{{=}0} ~dt~df~d\tau~d\nu \\ 
   {=} & \sum_n^N \lambda_n
\end{align}

\section{Implementation Supplement: MEM for MU-MIMO channels}

We analyze the proposed MEM and ZP-MEM for MU-MIMO non-stationary channels using 3GPP 38.901 UMa NLOS senario built on QuaDriga in Matlab. The channel parameters and the layout of the base station (BS) and the user equipment (UE) are shown in Table~\ref{tab:parameters}. 

\begin{table}[h]
\caption{Parameters of channel C}

\centering
\begin{tabular}{|c|c|}
\midrule
\textbf{Parameter} & \textbf{Value} \\ \midrule
Channel model & 3GPP 38.901 UMa NLOS \cite{3gpp.38.901}\\\midrule % 
Array type & BS: 3GPP 3-D \cite{3gpp.37.885}; UE: Vehicular \cite{3gpp.36.873} \\\midrule 
BS antenna & Height $h_b = 10$ m; Number $N_T = 4$ \\\midrule
UE antenna & Height $h_u = 1.5$ m; Number $M = 2$ \\\midrule
UE number & $K = 2$ \\\midrule
UE speed & $v \in [100, 150]$ km/h \\\midrule
% Initial distance & $100 \pm 10$ m \\\midrule
% Orientation & $\frac{3}{4}\pi$ \\\midrule
Bandwidth & Bw = $20$ Mhz     \\\midrule
Center frequency & $f_c = 5$ Ghz \\ \midrule
Subcarriers & $N_s = 64$ \\ \midrule

\end{tabular}
\label{tab:parameters}
\end{table}

Figure~\ref{fig:ber_c} and figure~\ref{fig:th_c} show the BER and throughput of MEM and ZP-MEM with QPSK, 16-QAN and 64-QAN modulations. BER of MEM is limited to around $10^{-2}$ as HoGMT decomposition for larger size (6-D) channels leads to more eigenwaves with low $\sigma_n$. Data symbols using those eigenwaves as carriers will suffer from strong noise enhancement after demodulation. ZP-MRC has lower BER as it doesn't use those eigenwaves. However, it means ZP-MEM doesn't fully leverage eigen diversity, which results in lower throughput than MEM. Overall, the performance of MEM and ZP-MEM for china C shows that MEM has generality to higher dimensional channels. On the other hand, OTFS requires additional precoding techniques to cancel spatial interference.   

\begin{figure}[t]
\begin{subfigure}{.24\textwidth}
  \centering
  \includegraphics[width=1\linewidth]{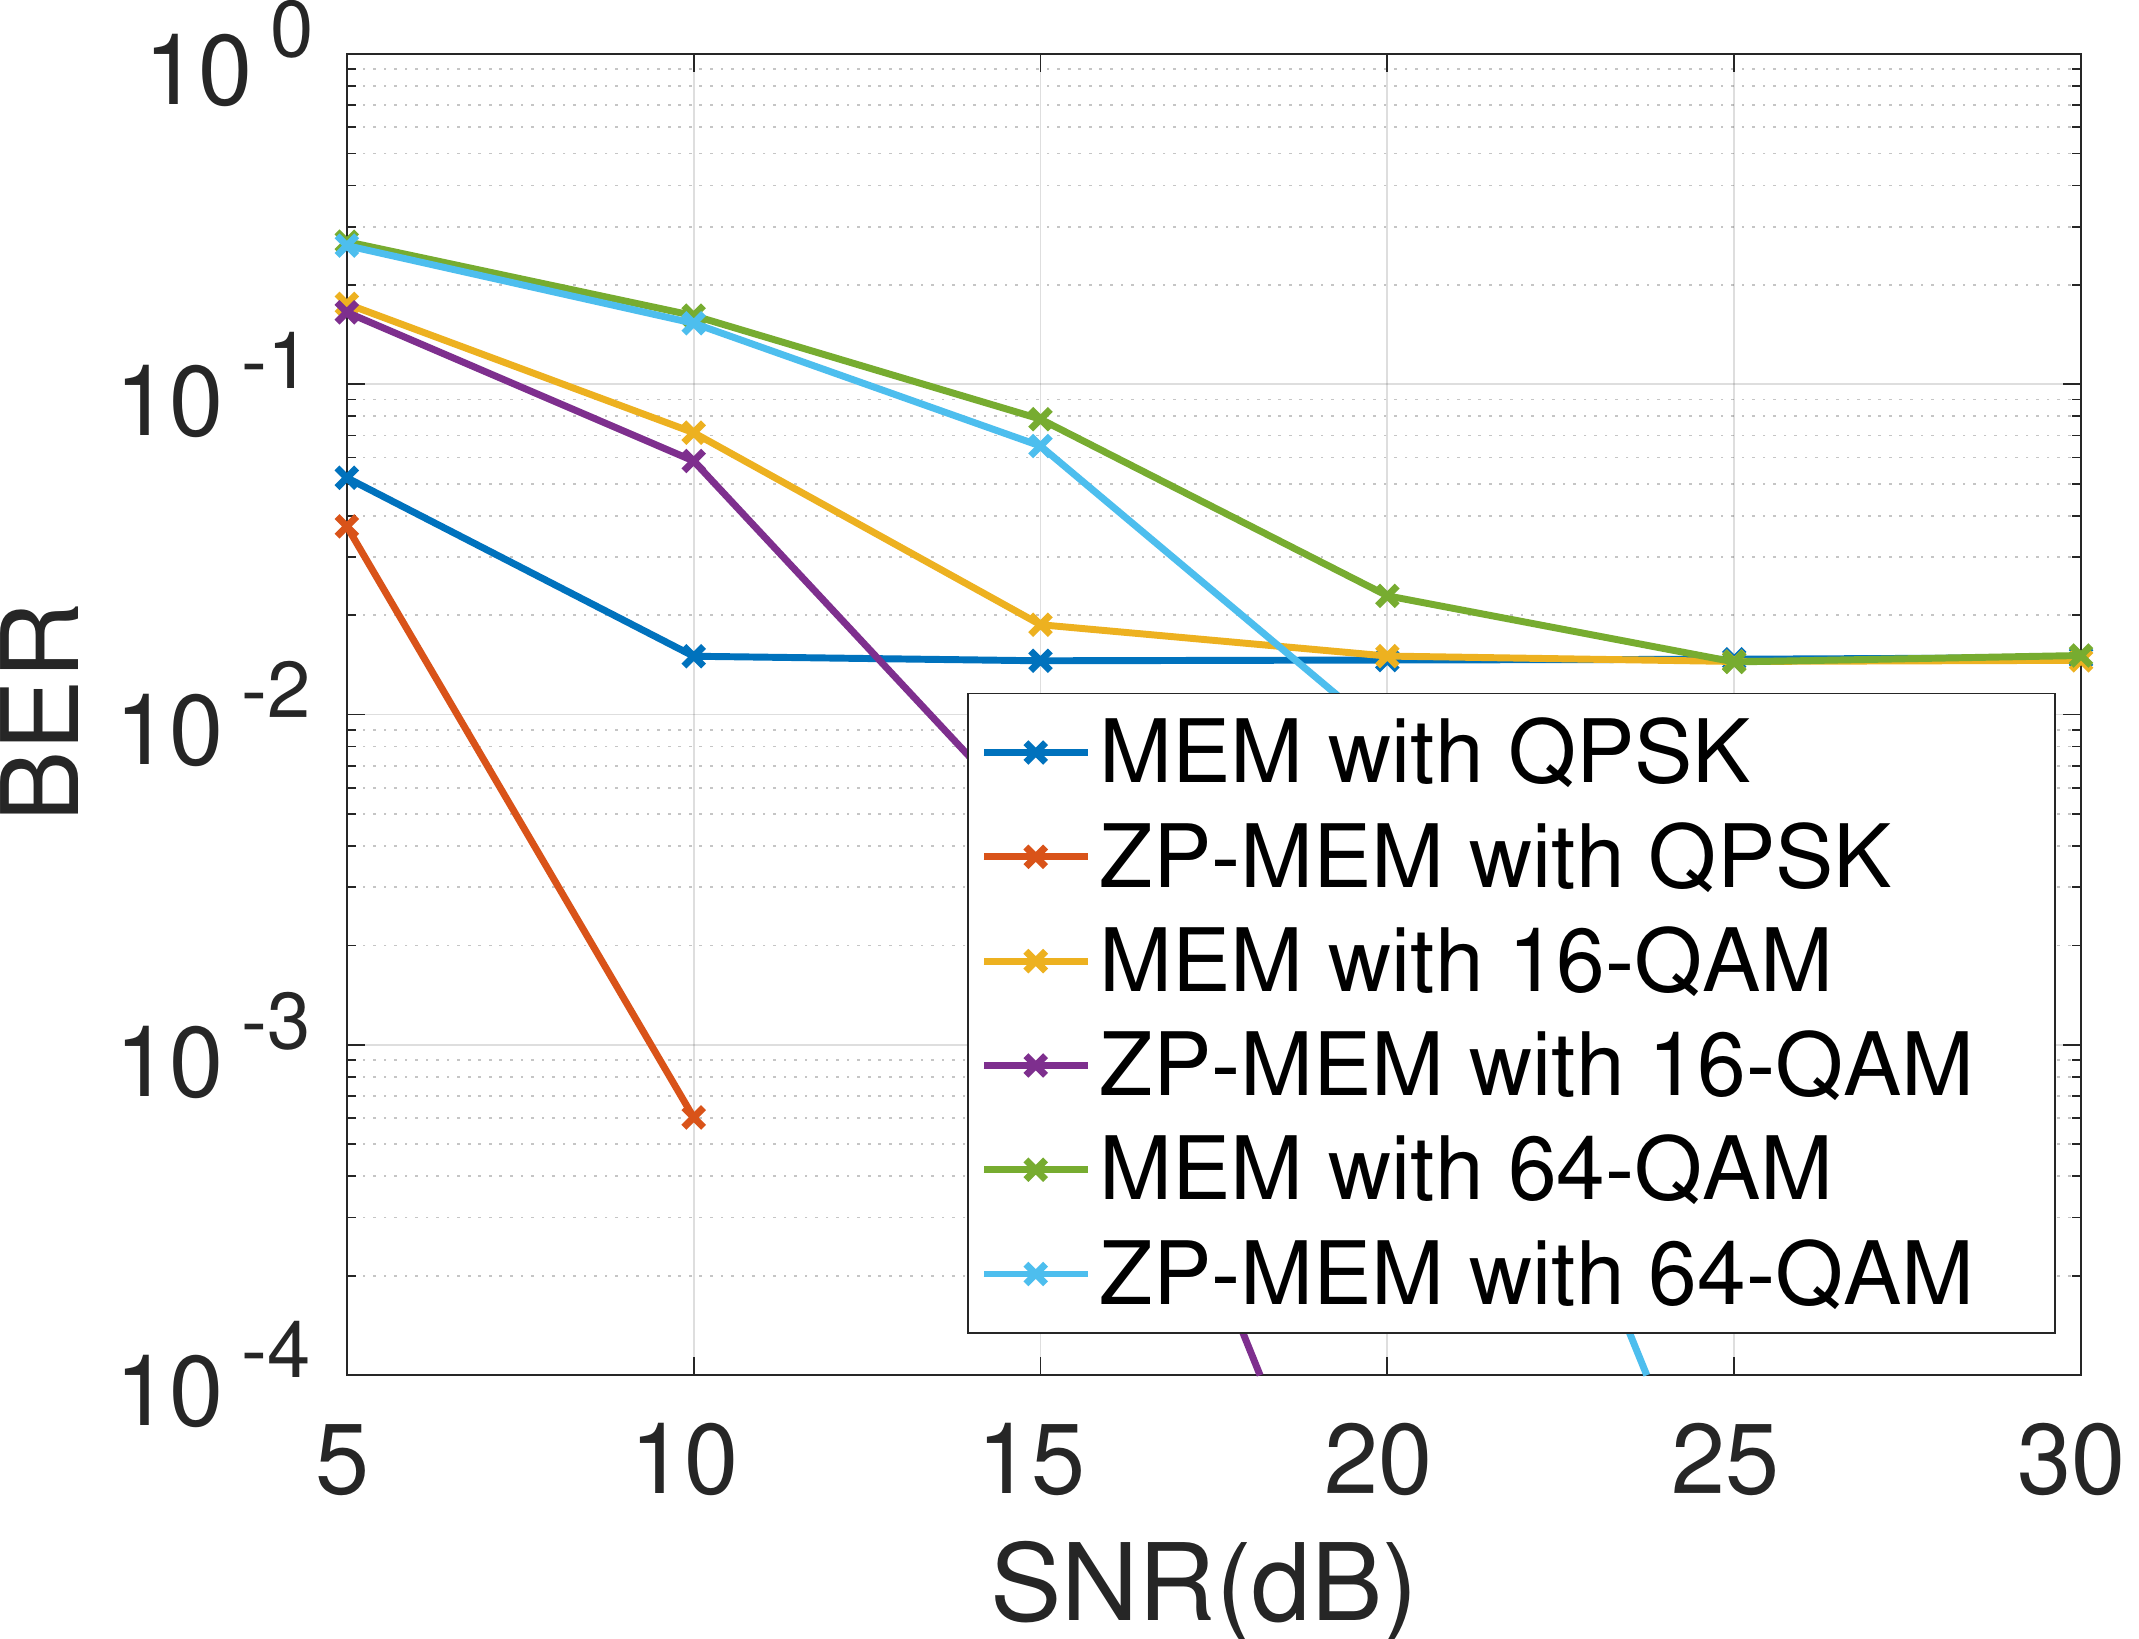}
  \caption{BER of MEM and ZP-MEM with QPSK, 16-QAM and 64-QAM
%   \note{Say absolute on y-axis.}
  } %at channel delay taps}
  \label{fig:ber_c}
\end{subfigure}
\begin{subfigure}{.24\textwidth}
  \centering
  \includegraphics[width=1\linewidth]{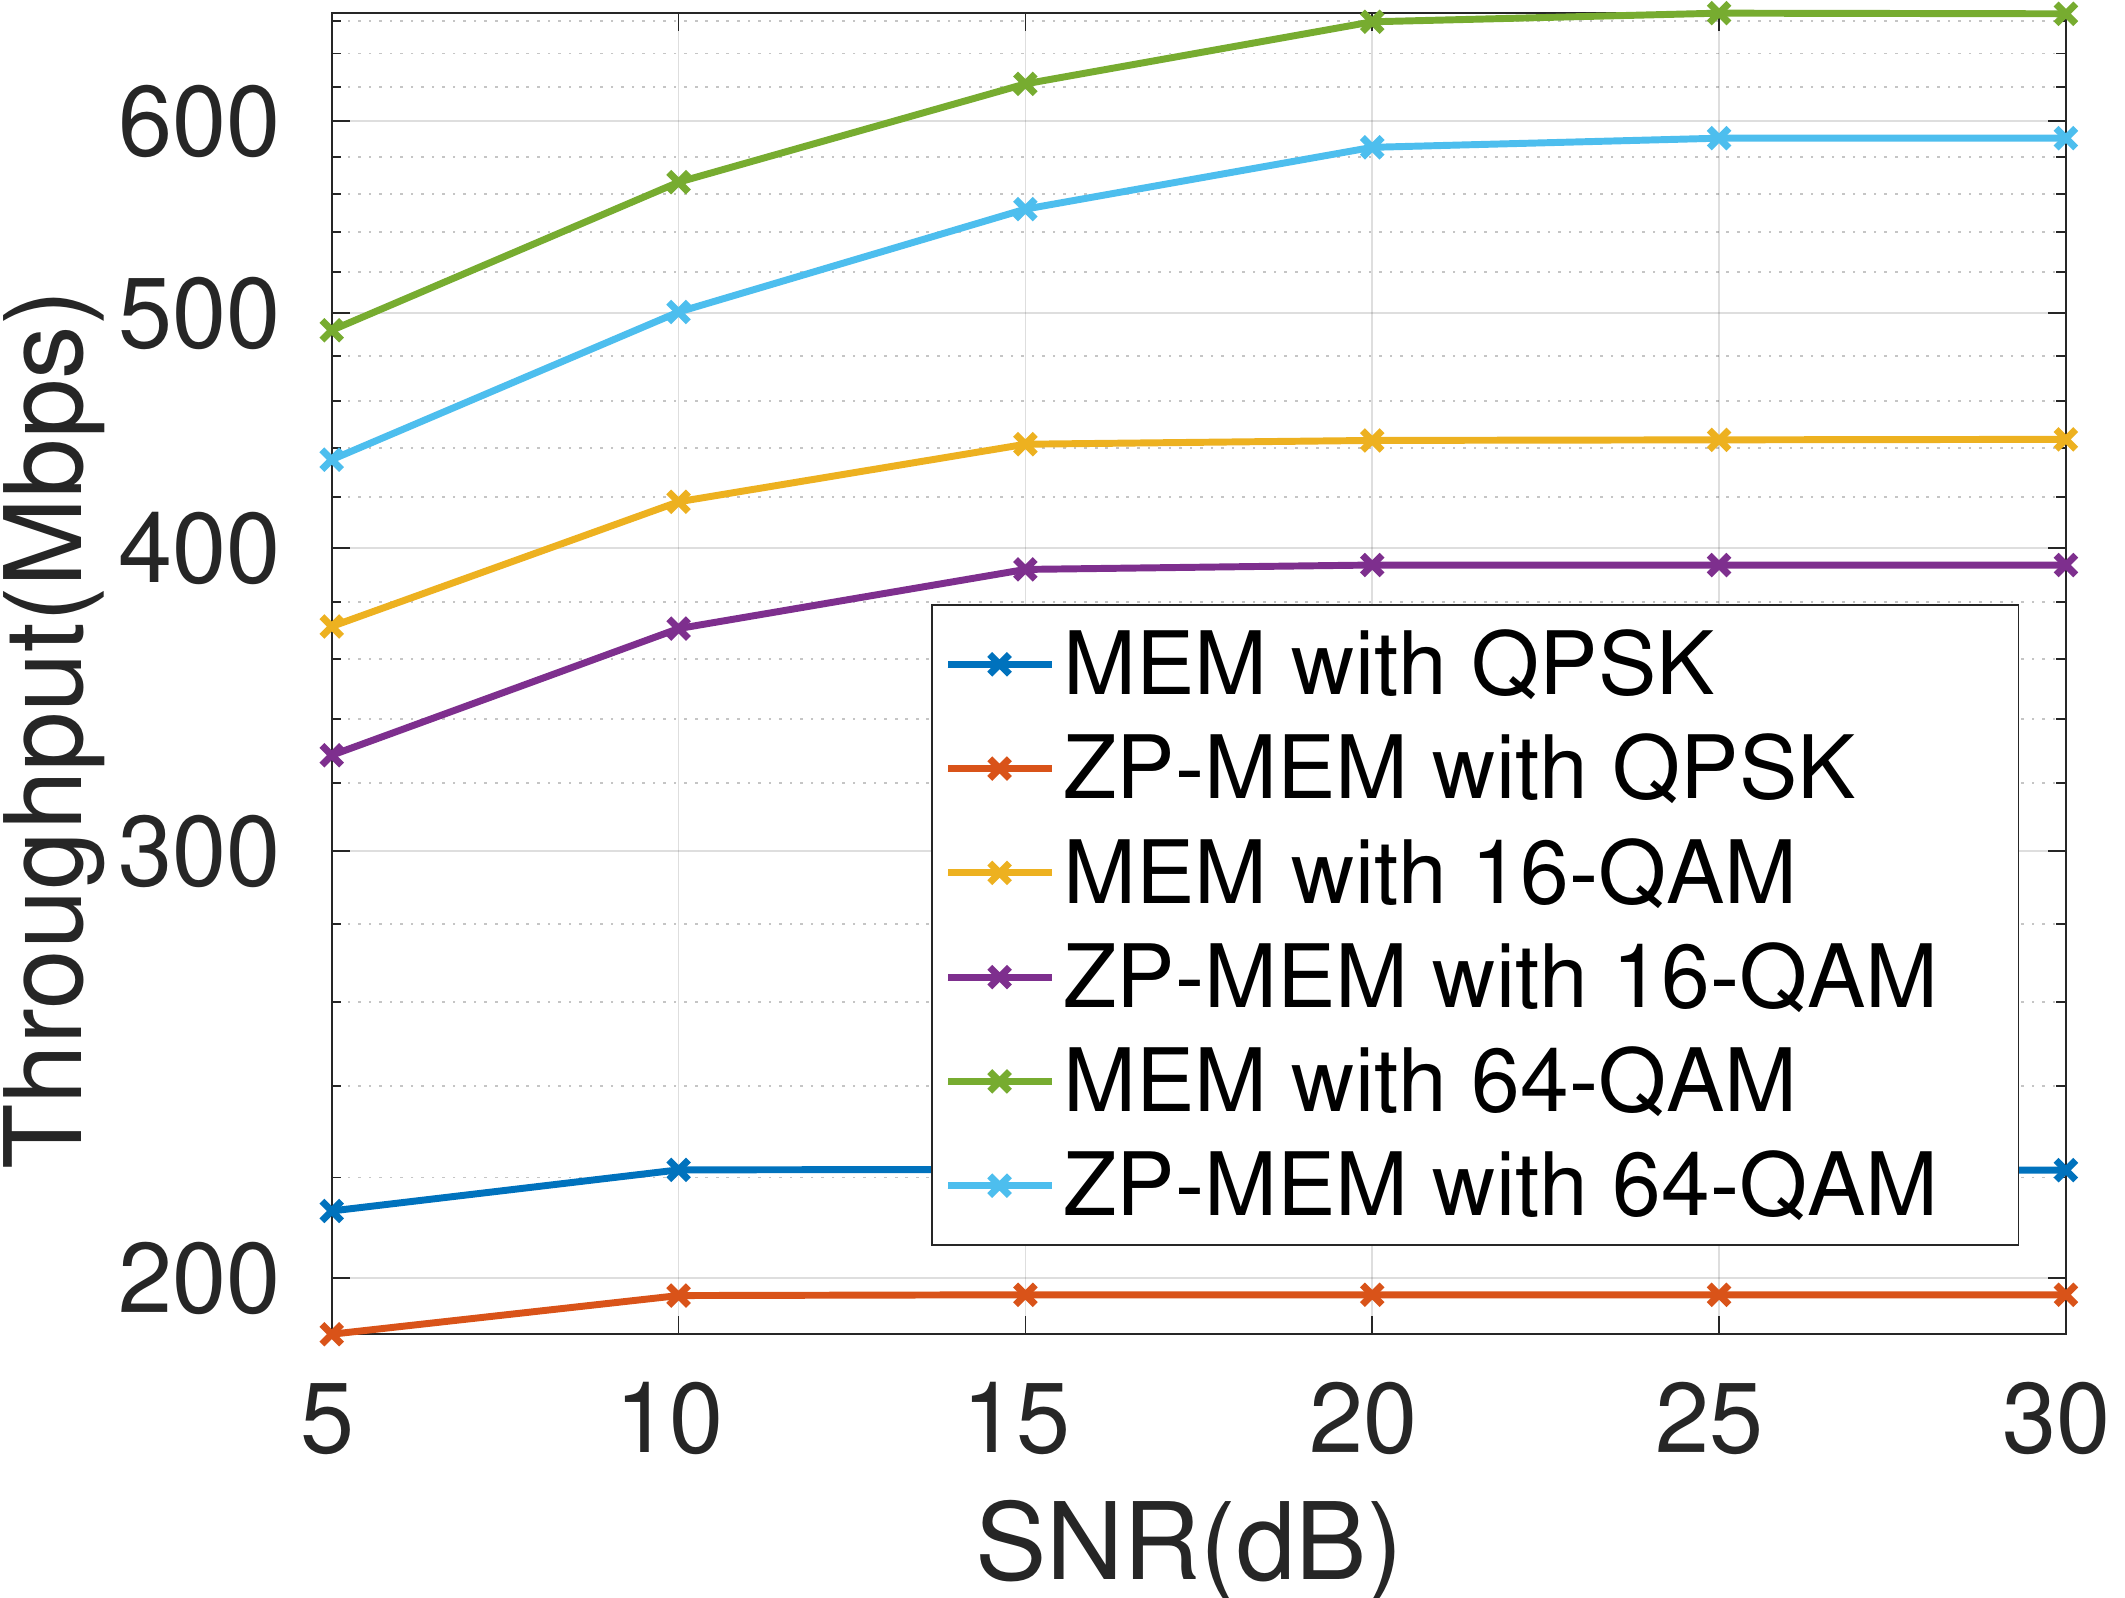}
  \caption{Throughput MEM and ZP-MEM with QPSK, 16-QAM and 64-QAM }
  \label{fig:th_c}
\end{subfigure}
  \caption{MEM and ZP-MEM for Channel C}
  \label{fig:cc}
\end{figure}
